# Supplementary material for: Tree-based boosting with functional data
Source: arXiv:2109.02989 source file (2023-04-06)
Supplement: Supplementary file 1 [file basis.tex]

To construct orthonormalized cubic B-spline for \texttt{TFBoost} from cubic B-spline, we referred to the procedure of Gram-Schimit orthonomalization \citep{de1968least}.

  Given a basis $\phi_1, ...,\phi_d$ (the cubic B-spline in our case) an orthonormal basis $\psi_1, ..., \psi_d$ can be constructed by successively solving a least-squared approximation problem  $d-1$ times: 
  \begin{align*}
\tilde{\psi}_i &= 	\phi_i - \sum_{j = 1}^{i-1} \langle \phi_i, \psi_j\rangle \psi_j \\
\psi_i &= \tilde{\psi}_i/||\tilde{\psi}_i||. 
  \end{align*}
  
 % where  $\psi_i$ is computed as the normalized vector of the best approximation to $\phi_i$ by elements in the space of $\phi_1,..., \phi_{i-1}$.
  
 In practice,  we adopted the modified Gram-Schimidt process which is computationally more stable:   for $i = 1,..., d$
 \begin{align*}
&\phi_i^{(1)}= \phi_i \\
&\phi_i^{(j+1)} = \phi_i^{(j)} - \langle \phi_i^{(j)}, \psi_j \rangle \psi_j, j = 1,..., i-1 \\
&\psi_i = \phi_i^{(i)}/||\phi_i^{(i)}||. 
  \end{align*}
Riemann integral with the mid-point rule was applied to calculate norms $||\cdot||$ and inner products $\langle \cdot, \cdot \rangle$.
