# Supplementary material for: Tree-based boosting with functional data
Source: arXiv:2109.02989 source file (2023-04-06)
Supplement: Supplementary file 4 [file sim_depth_select.tex]

% latex table generated in R 4.2.2 by xtable 1.8-4 package
% Fri Jan 13 00:13:32 2023
\begin{table}[H]
\centering
\begin{tabular}{rcccc}
  \hline
  & \multicolumn{2}{c}{SNR = 20} & \multicolumn{2}{c}{SNR = 5}\\ \hline
 & $M_1$ & $M_2$ & $M_1$ & $M_2$ \\ 
  TFBoost(A.1) & 1.590 (0.637) & 1.980 (0.876) & 1.580 (0.768) & 1.770 (0.983) \\ 
  TFBoost(A.2) & 1.440 (0.608) & 1.710 (0.844) & 1.550 (0.783) & 1.670 (0.965) \\ 
  TFBoost(A.3) & 1.540 (0.626) & 1.740 (0.787) & 1.400 (0.651) & 1.640 (0.823) \\ 
  TFBoost(B) & 1.510 (0.732) & 1.520 (0.659) & 1.320 (0.665) & 1.320 (0.601) \\ 
   \hline
\end{tabular}
\caption{Summary statistics of the depths selected by TFBoost methods for data generated from $r_1$; displayed in the form of mean (sd).} 
\end{table}
% latex table generated in R 4.2.2 by xtable 1.8-4 package
% Fri Jan 13 00:13:35 2023
\begin{table}[H]
\centering
\begin{tabular}{rcccc}
  \hline
  & \multicolumn{2}{c}{SNR = 20} & \multicolumn{2}{c}{SNR = 5}\\ \hline
 & $M_1$ & $M_2$ & $M_1$ & $M_2$ \\ 
  TFBoost(A.1) & 1.750 (0.716) & 2.170 (1.016) & 1.790 (0.832) & 2.200 (1.064) \\ 
  TFBoost(A.2) & 2.720 (0.805) & 2.850 (0.903) & 2.460 (1.086) & 2.350 (1.048) \\ 
  TFBoost(A.3) & 3.070 (0.820) & 2.950 (0.936) & 2.530 (1.049) & 2.350 (0.914) \\ 
  TFBoost(B) & 3.340 (0.685) & 2.660 (0.997) & 2.720 (1.055) & 1.990 (0.916) \\ 
   \hline
\end{tabular}
\caption{Summary statistics of the depths selected by TFBoost methods for data generated from $r_2$; displayed in the form of mean (sd).} 
\end{table}
% latex table generated in R 4.2.2 by xtable 1.8-4 package
% Fri Jan 13 00:13:37 2023
\begin{table}[H]
\centering
\begin{tabular}{rcccc}
  \hline
  & \multicolumn{2}{c}{SNR = 20} & \multicolumn{2}{c}{SNR = 5}\\ \hline
 & $M_1$ & $M_2$ & $M_1$ & $M_2$ \\ 
  TFBoost(A.1) & 1.160 (0.395) & 1.080 (0.273) & 1.390 (0.618) & 1.060 (0.239) \\ 
  TFBoost(A.2) & 1.810 (0.873) & 1.430 (0.573) & 1.880 (0.946) & 1.470 (0.731) \\ 
  TFBoost(A.3) & 1.800 (0.899) & 1.760 (0.878) & 1.810 (0.895) & 1.710 (0.856) \\ 
  TFBoost(B) & 2.970 (0.881) & 3.120 (0.729) & 2.220 (0.960) & 2.970 (0.881) \\ 
   \hline
\end{tabular}
\caption{Summary statistics of the depths selected by TFBoost methods for data generated from $r_3$; displayed in the form of mean (sd).} 
\end{table}
% latex table generated in R 4.2.2 by xtable 1.8-4 package
% Fri Jan 13 00:13:40 2023
\begin{table}[H]
\centering
\begin{tabular}{rcccc}
  \hline
  & \multicolumn{2}{c}{SNR = 20} & \multicolumn{2}{c}{SNR = 5}\\ \hline
 & $M_1$ & $M_2$ & $M_1$ & $M_2$ \\ 
  TFBoost(A.1) & 2.190 (0.787) & 1.980 (0.512) & 2.100 (0.835) & 1.740 (0.661) \\ 
  TFBoost(A.2) & 2.580 (0.713) & 2.400 (0.620) & 2.220 (0.938) & 2.210 (0.913) \\ 
  TFBoost(A.3) & 2.500 (0.689) & 2.470 (0.674) & 2.150 (0.914) & 2.120 (0.891) \\ 
  TFBoost(B) & 3.060 (0.789) & 2.450 (0.687) & 2.850 (0.947) & 2.300 (0.859) \\ 
   \hline
\end{tabular}
\caption{Summary statistics of the depths selected by TFBoost methods for data generated from $r_4$; displayed in the form of mean (sd).} 
\end{table}
% latex table generated in R 4.2.2 by xtable 1.8-4 package
% Fri Jan 13 00:13:42 2023
\begin{table}[H]
\centering
\begin{tabular}{rcccc}
  \hline
  & \multicolumn{2}{c}{SNR = 20} & \multicolumn{2}{c}{SNR = 5}\\ \hline
 & $M_1$ & $M_2$ & $M_1$ & $M_2$ \\ 
  TFBoost(A.1) & 3.030 (0.881) & 3.330 (0.792) & 2.570 (1.066) & 3.050 (0.892) \\ 
  TFBoost(A.2) & 2.630 (0.861) & 3.220 (0.883) & 2.230 (0.973) & 2.610 (1.004) \\ 
  TFBoost(A.3) & 2.340 (0.855) & 3.200 (0.725) & 1.940 (0.814) & 2.600 (0.964) \\ 
  TFBoost(B) & 1.590 (0.712) & 2.250 (1.019) & 1.430 (0.590) & 1.790 (0.782) \\ 
   \hline
\end{tabular}
\caption{Summary statistics of the depths selected by TFBoost methods for data generated from $r_5$; displayed in the form of mean (sd).} 
\end{table}
